# Supplementary material for: Temporally Multi-Scale Sparse Self-Attention for Physical Activity Data Imputation
Source: arXiv:2406.18848 source file (2024-06-27)
Supplement: Supplementary file 1 [file 11appendix_long.tex]

%\section{First Appendix}\label{apd:first}

% \documentclass[twoside]{article}

% \usepackage{aistats2024}
% \usepackage{caption}
% \usepackage{subcaption}
% \usepackage{graphicx} 
% \usepackage{amssymb}
% \usepackage{xcolor}
% \usepackage{booktabs}
% \usepackage[ruled, linesnumbered]{algorithm2e}

% If your paper is accepted, change the options for the package
% aistats2022 as follows:
%
%\usepackage[accepted]{aistats2024}
%
% This option will print headings for the title of your paper and
% headings for the authors names, plus a copyright note at the end of
% the first column of the first page.
\clearpage

\section{Data Curation and Preprocessing Pipeline} \label{sec:curation_preprocess}

We would like to clarify that we are \textbf{NOT} redistributing or publish any data or statistics with the intent of reproducing the \textit{All of Us} Research Program database or part of the database outside of the \textit{All of Us} Researcher Workbench. Instead, our intent is for researchers to register for \textit{All of Us} account and then use our preprocessing codes to reproduce the cohort \textbf{within} the \textit{All of Us} Research Workbench.

%\vspace{3cm}

\begin{figure}[ht!]
\centering
\includegraphics[width=\columnwidth]{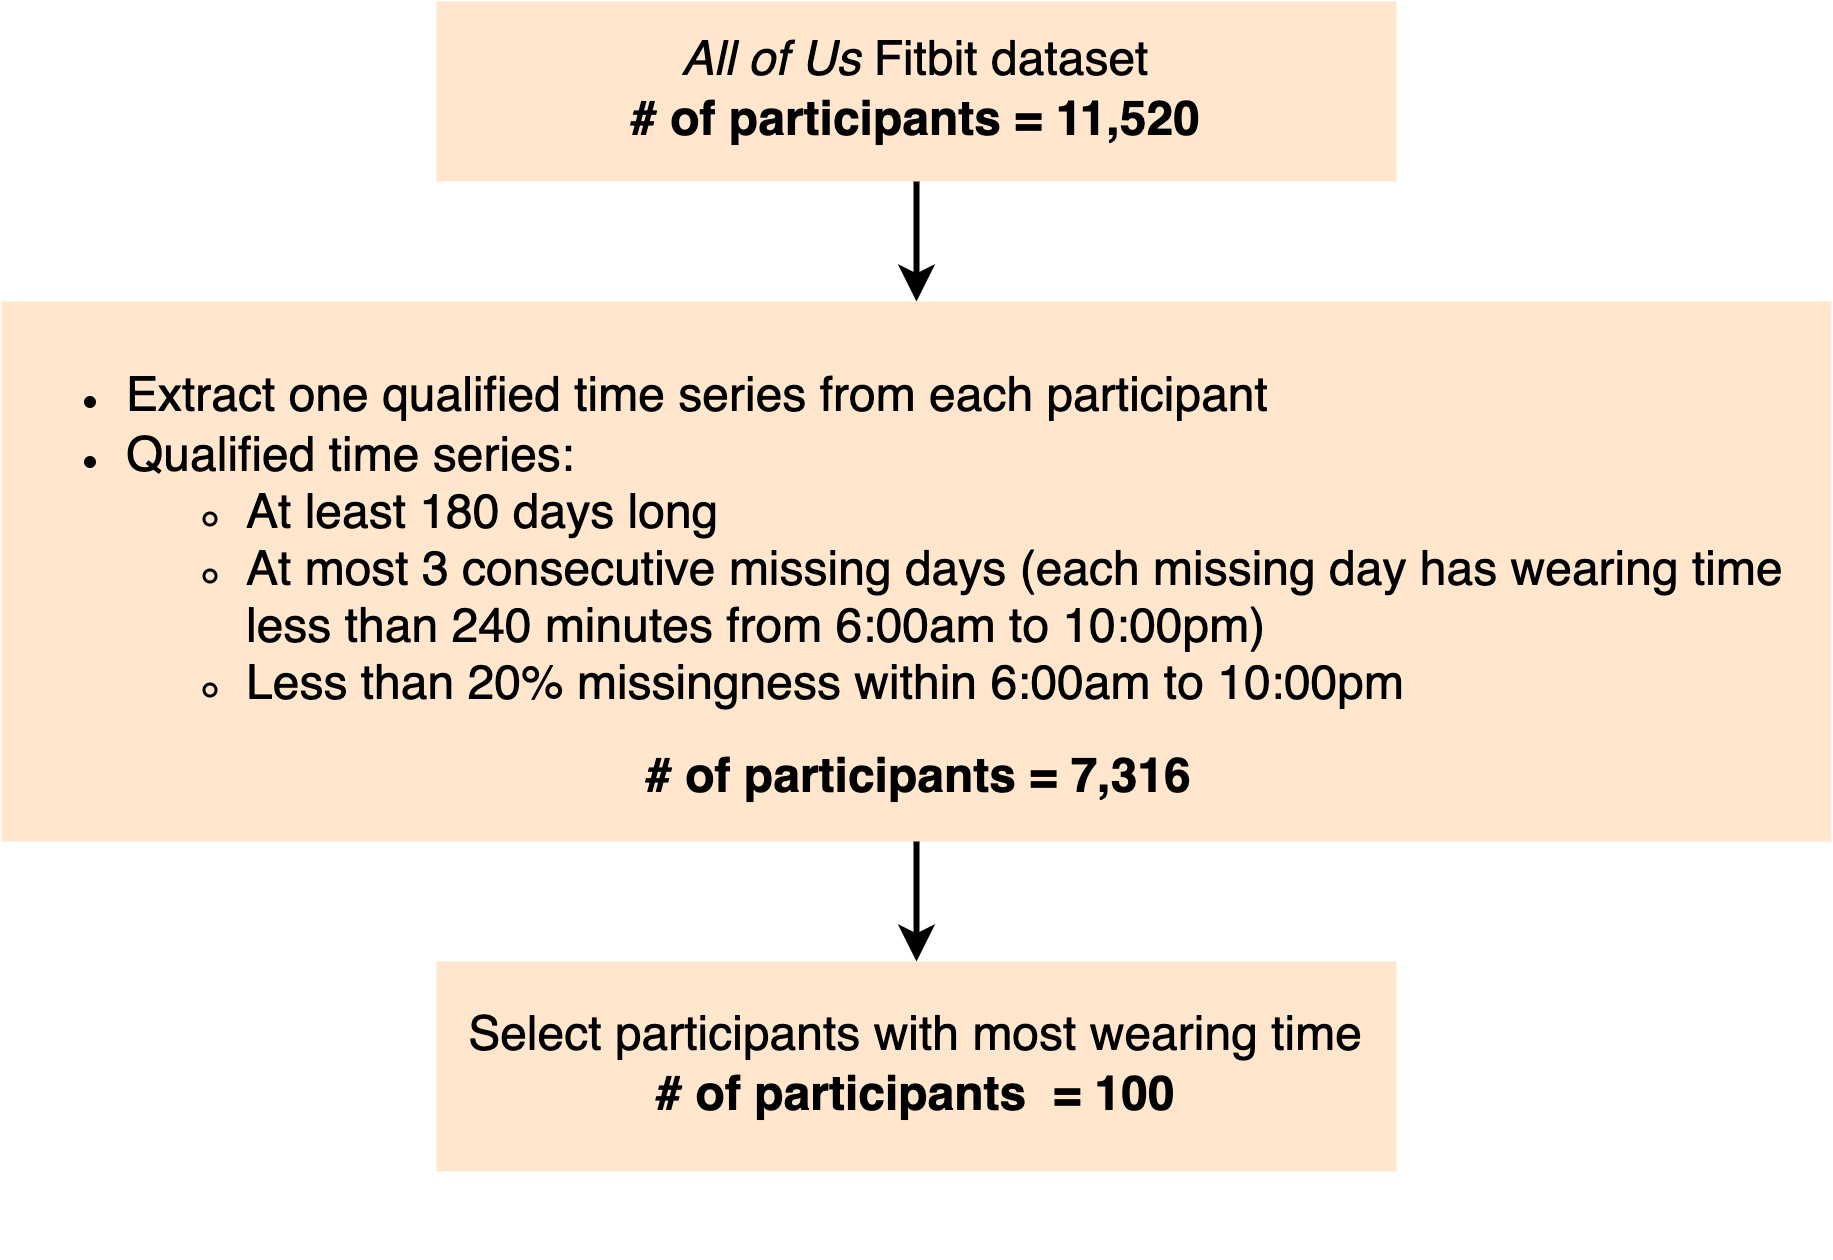}
\caption{Flow chart for cohort curation}
\label{fig:cohort_describe}
\end{figure}

\begin{figure}[!htb]
\centering
\includegraphics[width=\columnwidth]{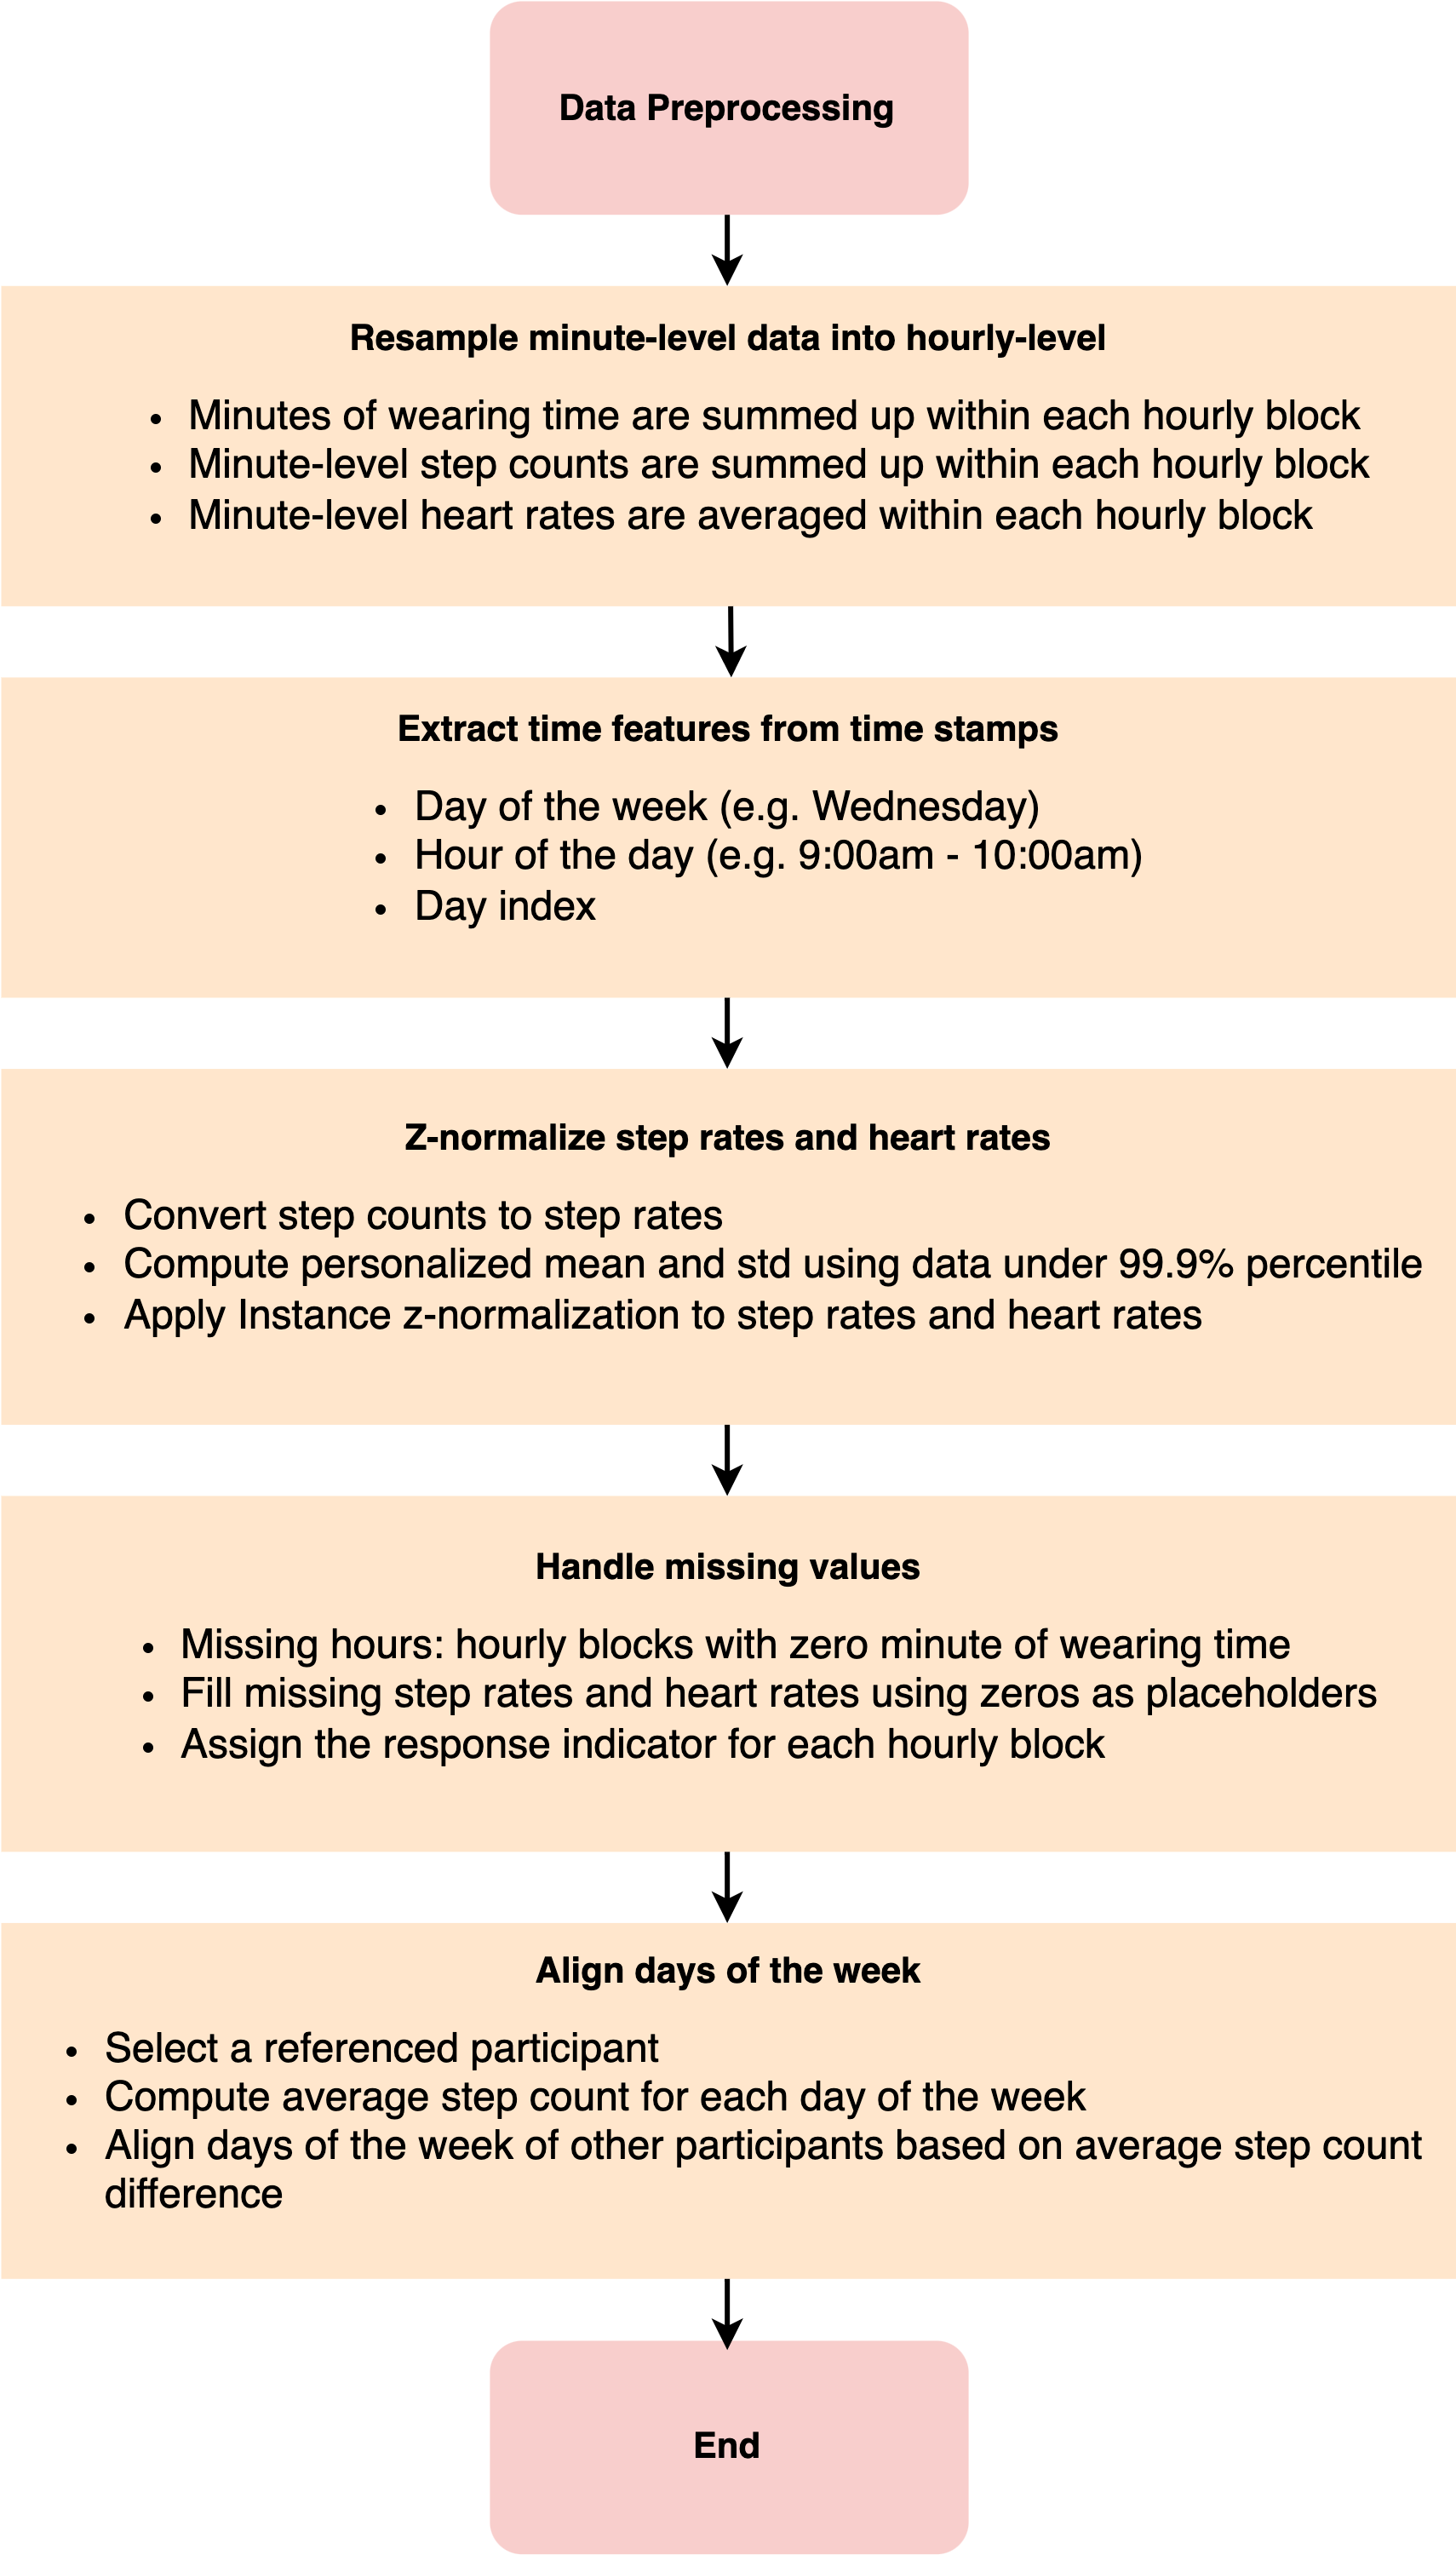}
\caption{Data preprocessing pipeline}
\label{fig:data_preprocessing}
\end{figure}

%\clearpage

\section{Comparison between Curated Cohort and All \textit{All of Us} Participants} \label{sec:comp_cohort_allofus}

To compare our curated cohort with 100 participants and the entire \textit{All of Us} Fitbit dataset with 11,520 participants,  we draw the histogram of (1) total number of hourly blocks, (2) total number of valid hourly blocks (i.e. have at least one minute of wearing time), (3) missing rate between 6am to 10pm in \figureref{fig:stats_basic}, as well as (4) participant level average heart rates and hourly block step rates, (5) hourly step rates for each hourly of the day and (6) missing rate of each hour of the day from 0am to 11pm in \figureref{fig:stats_hr_sr_miss}.

% \begin{figure*}[htp!]
% \centering
% \includegraphics[height=3cm, width=\linewidth, keepaspectratio]{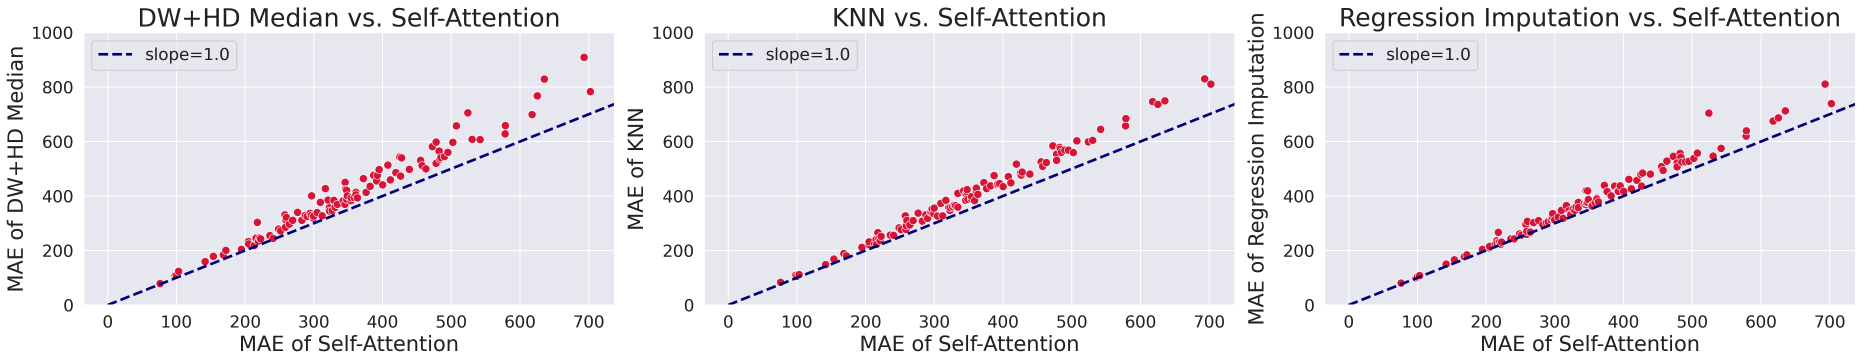}
% \caption{Model comparison on the participant level between baselines and our self-attention model. Each point shows the performance of different models on different axes. The results are averaged over 10 splits. The reference line with slope 1.0 indicates two model have the same performance.}

% \label{fig:model_compare_participant}
% \end{figure*}

\begin{figure*}[htbp!]
\floatconts
  {fig:stats_basic}
  {\caption{\textbf{Blue}: Statistics of the entire \textit{All of Us} Fitbit dataset with 11,520 participants. \textbf{Orange}: Statistics of our curated cohort with 100 participants. \textbf{First column}: Distribution of the total number of hourly blocks from each participant. \textbf{Second column}: The total number of valid hourly blocks (i.e. hourly blocks with non-zero wearing minutes) from each participant. \textbf{Third column}: Missing rate (i.e. the number of invalid hourly blocks divided by the total number of hourly blocks), including all hours of the day, not only from 6:00 to 22:00, of each participant. }}
  {%
    \subfigure[The entire \textit{All of Us} dataset]{\label{fig:entire_basic}%
      \includegraphics[width=\linewidth]{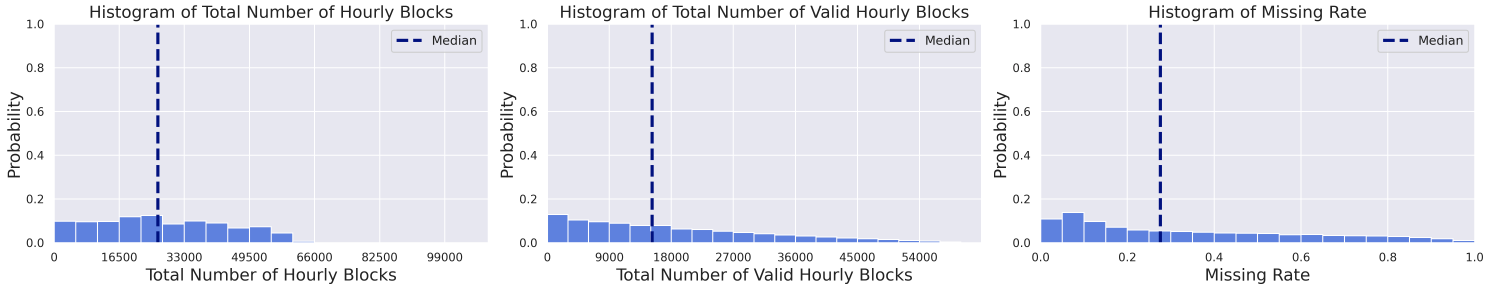}}%
    \qquad
    \subfigure[Our cohort]{\label{fig:top_basic}%
      \includegraphics[width=\linewidth]{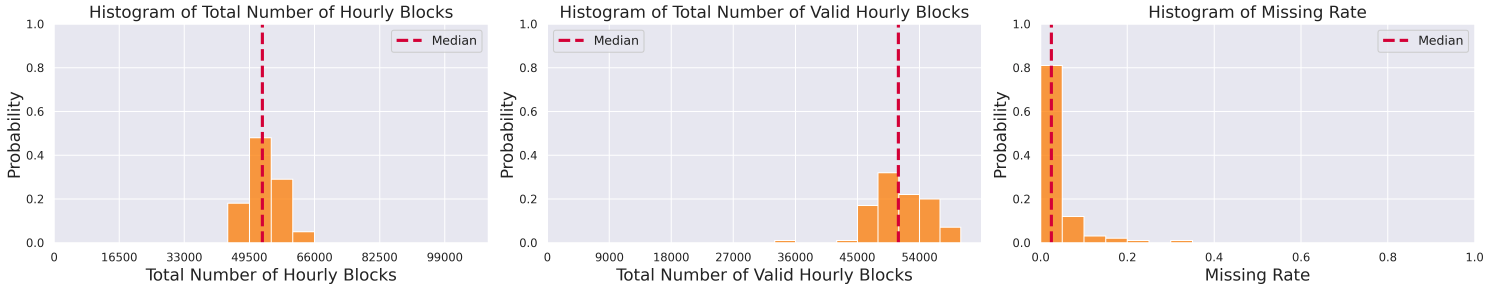}}
  }
\end{figure*}

% \begin{figure*}[ht!]
% \centering
% \begin{subfigure}[b]{1\linewidth}
%    \includegraphics[width=1\linewidth]{images/entire_dataset_basic_stats.png}
%    %\caption{}
%    \label{fig:entire_basic} 
% \end{subfigure}

% \begin{subfigure}[b]{1\textwidth}
%    \includegraphics[width=1\textwidth]{images/top_cohort_basic_stats.png}
%    %\caption{}
%    \label{fig:top_basic}
% \end{subfigure}
% \caption{\textbf{Blue}: Statistics of the entire \textit{All of Us} Fitbit dataset with 11,520 participants. \textbf{Orange}: Statistics of our curated cohort with 100 participants. \textbf{First column}: Distribution of the total number of hourly blocks from each participant. \textbf{Second column}: The total number of valid hourly blocks (i.e. hourly blocks with non-zero wearing minutes) from each participant. \textbf{Third column}: Missing rate (i.e. the number of invalid hourly blocks divided by the total number of hourly blocks), including all hours of the day, not only from 6:00 to 22:00, of each participant. } 
% \end{figure*}

%\vfill

\begin{figure*}[htbp!]
\floatconts
  {fig:stats_hr_sr_miss}
  {\caption{\textbf{Blue}: Statistics of the entire \textit{All of Us} Fitbit dataset with 11,520 participants. \textbf{Orange}: Statistics of our curated cohort with 100 participants. \textbf{First column}: Distribution of average heart rates over all the participants. \textbf{Second column}: Distribution of average hourly step rates over all the participants. \textbf{Third column}: Distribution of hourly step rates of each hour of the day. \textbf{Fourth column}: Missing rate of each hour of the day. The average heart rates and average step rates are computed over all the hourly blocks with non-zero wearing minutes for each participant.}}
  {%
    \subfigure[The entire \textit{All of Us} dataset]{\label{fig:entire_hr_sr_miss}%
      \includegraphics[width=\linewidth]{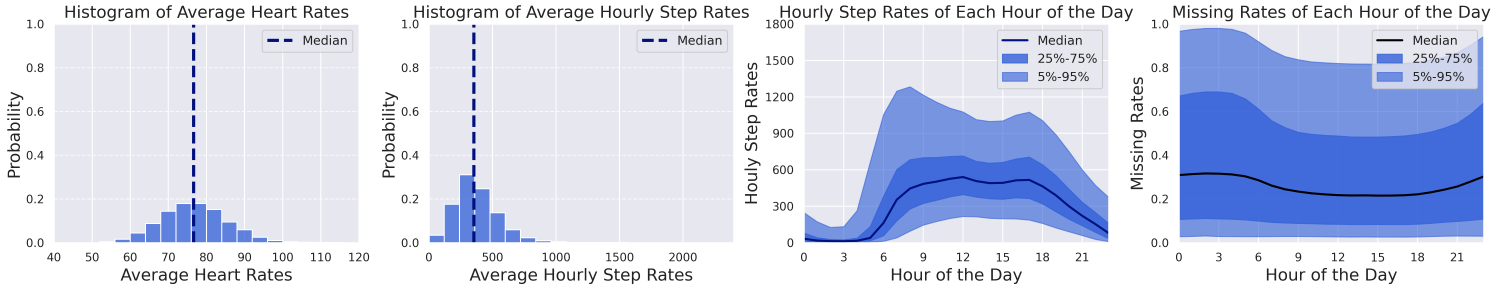}}%
    \qquad
    \subfigure[Our cohort]{\label{fig:top_hr_sr_miss}%
      \includegraphics[width=\linewidth]{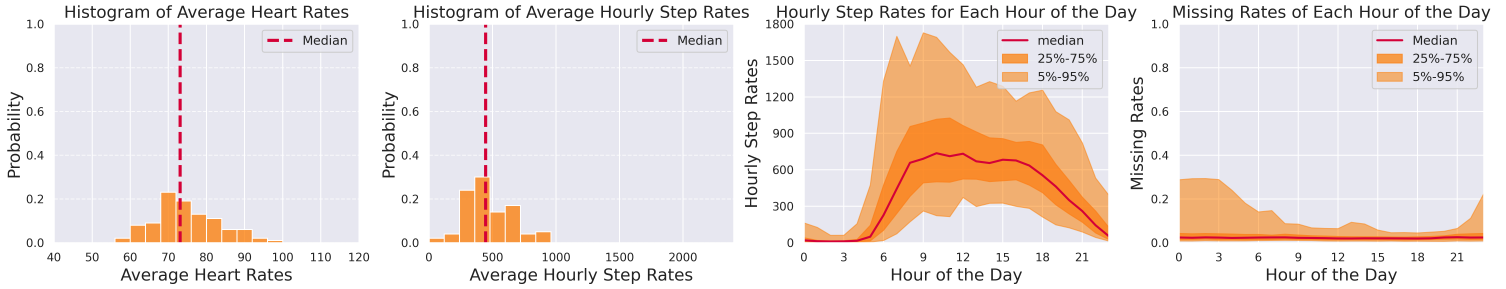}}
  }
\end{figure*}

% \begin{figure*}[ht!]
% \centering
% \begin{subfigure}[b]{1\textwidth}
%    \includegraphics[width=1\linewidth]{images/entire_dataset_hr_sr_miss.png}
%    %\caption{}
%    \label{fig:entire_basic} 
% \end{subfigure}

% \begin{subfigure}[b]{1\textwidth}
%    \includegraphics[width=1\linewidth]{images/top_cohort_hr_sr_miss.png}
%    %\caption{}
%    \label{fig:top_basic}
% \end{subfigure}
% \caption{\textbf{Blue}: Statistics of the entire \textit{All of Us} Fitbit dataset with 11,520 participants. \textbf{Orange}: Statistics of our curated cohort with 100 participants. \textbf{First column}: Distribution of average heart rates over all the participants. \textbf{Second column}: Distribution of average hourly step rates over all the participants. \textbf{Third column}: Distribution of hourly step rates of each hour of the day. \textbf{Fourth column}: Missing rate of each hour of the day. The average heart rates and average step rates are computed over all the hourly blocks with non-zero wearing minutes for each participant.}

% \end{figure*}

%\clearpage

\section{Model Configurations, Hyperparameters and Training Procedures} \label{sec:model_setups}
In this section, we introduce the details about all the models used in our experiments, including their configurations, hyperparameters and training procedures.  

\subsection{Multi-Timescale Sparse Self-Attention Model}
For the context window, we set the number of hours on each side of the imputing hourly block as 4 and search for the number of weeks on each side within \{1, 2, 3, 4, 5\}. We found the best number of weeks is 5, and beyond 5 the performance gain is neglected. Therefore, since the first week is always full, the context window size in our case is $kh=2\times4+1 = 9$ and $kw=2\times(7+4)+1=23$.

\begin{figure}[ht]
\centering
\includegraphics[width=\columnwidth]{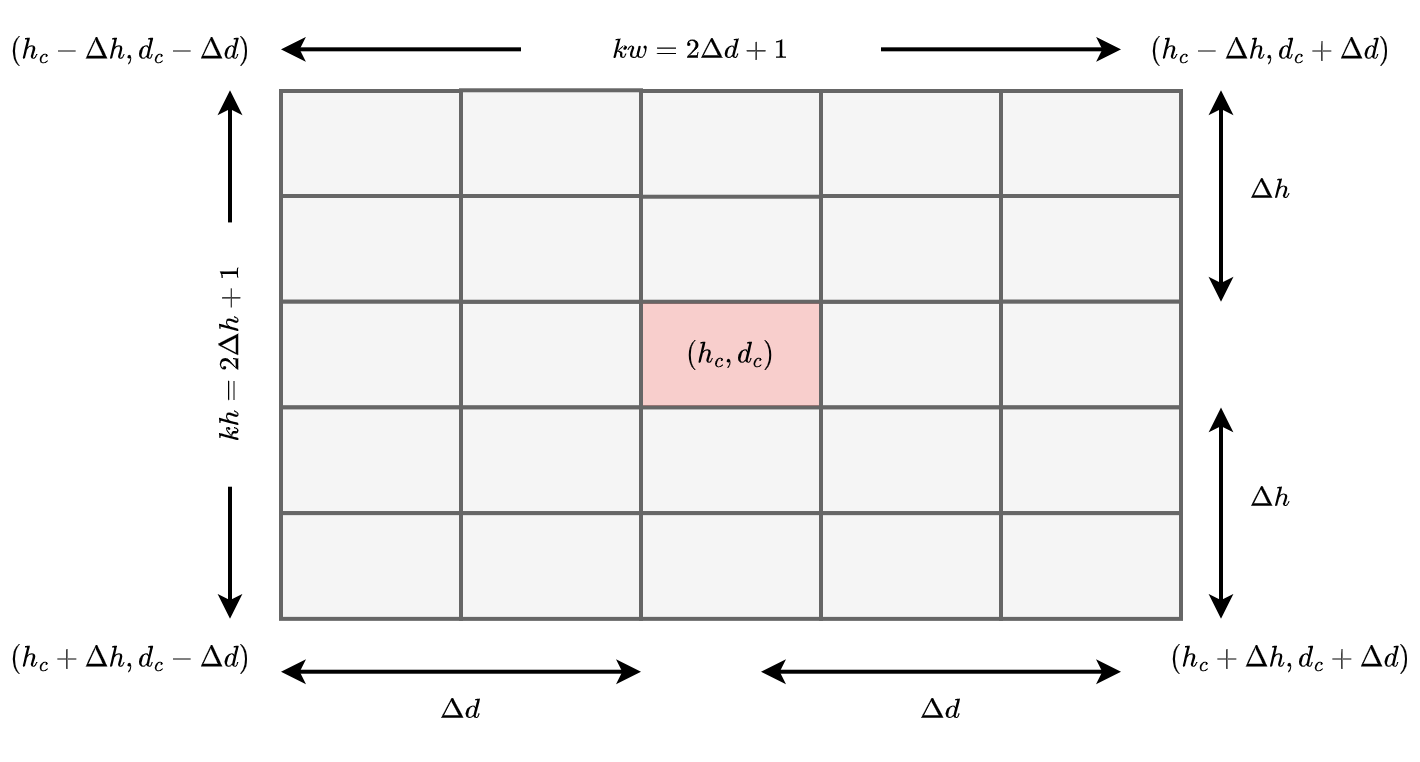}
\caption{Context window for the multi-timescale sparse self-attention model. In the experiment, we set $\Delta h = 4$ and $\Delta d = 7 + 4 = 11$. Therefore, the context window size is $kh \times kw = (2\Delta h+1) \times (2\Delta w + 1) = 9 \times 23$.} 
\label{fig:context_window}
\end{figure}

For local activity profile representations, we set its length as $2W+1 = 2\times72+1 = 145$. We fill missing values using the median step rate of day of the week and hour of the day (i.e. DW+HD Median). To prevent data leakage, we set as missing all positions in local activity representations that contain the ground-truth value of the center hourly block of the local context window, which is we are imputing for. Also, the model contains three identical encoding modules: $Conv \to LayerNorm \to ReLU \to Average Pool$, one for each of query, key and value. The configuration of the $Conv$ layer is: out\_channels=1, kernel\_size=49, stride=1, padding=24 and no bias. The kernel size and stride of $Average Pool$ is set as 7 and 6, respectively. 

As for input features, we include one-hot vectors for day of the week and hour of the day indicators in query, key, and value. Furthermore, we observe incorporating normalized step rates of the corresponding hourly block into query and value, along with adding normalized heart rates to value, can enhance the performance. The encoded local activity profile representation is concatenated with other input features. We use three linear layers to map input features to $\mathbf{q}$, $\mathbf{k}$ and $v$. We search for $d_k$ within \{4, 8, 16\}. 

During training, we use the Adam optimizer with batch size of 20,000 and search for learning rate within \{0.1, 0.01, 0.001\}. The best learning rate is 0.01 and the number of training epochs is set as 30. We conduct early stopping based on validation Micro MAE for each split. Also, average validation Micro MAE over 10 splits is used to choose the best hyperparameters. We train the model using two NVIDIA Tesla T4 GPUs with 32 CPUs and 208 RAM memory within \textit{All of Us} workspace. We implement the model using PyTorch 1.13.1.

\subsection{Filling Methods} 
All the filling methods impute missingness on the level of \emph{unnormalized} step rates (i.e. before instance z-normalization). Also, as mentioned in the loss function section, the predicted step rate will go through a non-linearity to limit the upper and lower bound of step rates and will be converted back to step counts using hourly wearing minutes to report the performance. All the filling methods leverage personal statistics, which means all the statistics (e.g. mean and median) are computed specifically from each participant, when filling missing values within that participant. When computing the mean and median w.r.t each factor (e.g. day of the week), all the test hourly blocks are removed to avoid the data leakage. For forward and backward based fillings, during testing, the imputing test hourly block can be filled with the ground-truth value of the other test hourly block if they are contiguous. More details of each filling method are as follows.

\begin{itemize}
    \item \textbf{Zero Fill}: fill missing step rates as zeros. This means when a hourly block has zero wearing minutes, we consider there is no physical activity. 
    
    \item \textbf{Micro Mean Fill}: we define the \emph{micro mean} step rate as the total number of step counts divided by the total number of wearing minutes in all the hourly blocks regarding: each participant, each day of the week, each hour of the day, or each combination of day of the week and hour of the day (e.g. 8am on Mondays). The factors are shared with mean fill and median fill methods. Also, since we only care about 6:00 to 22:00, all the statistics are calculated using data within this period.
    
    \item \textbf{Mean Fill}: we compute the mean step rate by computing the uniform mean over all the step rates from hourly blocks with non-zero wearing minutes. 
    
    \item \textbf{Median Fill}: we compute the median step rate by calculating the median over all the step rates from hourly blocks with non-zero wearing minutes.
    
    \item \textbf{Forward and Backward Fill}: different from above filling methods, all the data out of 6:00 to 22:00 are utilized when conducting forward and backward fillings. If there are still missing steps after fillings (e.g. all the hourly blocks are missing before 10:00, then after forward fill, they still remain missing), then they will be filled by the median step rate computed from all the participant non-missing hourly blocks. When computing the average of the forward and backward fill (Avg.F+B), if the results after either forward or backward fill still have the missing step rates, we use the results from the other method to fill. 
    
    %If a hourly block keeps still missing using both forward and backward fill, we use the participant median step rate to fill. 
\end{itemize}

\subsection{Regression Imputation}  
We use the linear regression model to impute missing step counts for this method. Input features of the linear regression model for each missing hourly block consists of: (1) normalized step rates and heart rate from all the hourly blocks in the context window, except for the center one, which is under imputation, (2) one-hot vectors of day of the week and hour of the day from the currently imputing center hourly block. \textcolor{red}{LAPR is not applied as it was found to decrease  performance.}

We fill missing step rates and heart rates in the context window by zeros. \textcolor{red}{Additionally, we conducted an evaluation of the DW+HD median method for handling missing data. However, our findings indicate that it exhibits inferior performance compared to the zero-imputation approach.} The linear regression model has the same context window size, training protocol and loss function as the sparse self-attention model. We set the batch size as 50,000 and search for the learning rate in $\{0.1, 0.01, 0.001, 0.0001\}$ and use Adam optimizer to train the model for 20 epochs with the learning rate of 0.001. 

\subsection{$k$-Nearest Neighbors ($k$NN) Imputations}
We search for nearest neighbors for each missing hourly block within all the non-missing hourly data, including those outside 6:00 to 22:00, from the \emph{same} participant data containing the missing hourly block. The feature of hourly blocks is all the step rates within $W$ hours on each side (same as the local activity profile representation in the self-attention model), resulting in the total dimension of $2W + 1$. Missing hourly blocks and the center hourly block within this $2W + 1$ window are filled with the median step rate w.r.t the day of the week and hour of the day (DW+HD median). 

Two $k$-NN variations are tested: (1) uniform averaging ($k$NN-Uniform) and (2) weighted averaging ($k$NN-Softmax) based on RBF kernel and the square distance between the imputing hourly block and its neighbors in the $2W+1$ feature space. Mathematically, let $\mathcal{N}$ denote the set of nearest neighbors of the missing hourly block $t'$ where $|\mathcal{N}|=K$. Let $\mathtt{B}(t',t): \mathcal{T} \times \mathcal{T} \to \mathbb{R}^{\geq 0}$ be the function to return the square distance in the feature space between $t'$ and $t$, then two variations are defined in the following equations:

\begin{equation}
\label{equ:mae}
s_{t'} = \frac{1}{K} \sum_{t \in \mathcal{N}} s_{t}, 
s_{t'} = \sum_{t \in \mathcal{N}}\frac{\exp(\mathtt{B}(t',t) / \tau)}{\sum_{u \in \mathcal{N}} \exp(\mathtt{B}(t',u)/ \tau)} s_{t}
\end{equation}

where $s_{t}$ is the step rate at time $t$. Then we use the same procedure to convert it back to the step count. In experiments, we set $W=72$, which is the same as the local physical activity profile representation dimension in the self attention model. We search for $K$ in \{1, 7, 14, 21, 28, 35\} for both variations and search for the RBF parameter $\tau$ in \{0.1, 0.01, 0.001, 0.0001, 0.00001\} for $k$NN-Softmax.

\subsection{Multiple Iterative Imputation Methods (Iterative Imputation)}
We implement a similar idea as Multiple Imputation with Chained Equations (MICE) method, which uses chained equations to impute every variable conditioned on the others for multiple iterations. However, during the training phase, the algorithm performs a deterministic imputation for each variable instead of probabilistic sampling. 

When training the model, we create the same local context window as used in the self-attention model. Each window is centered at each training instance and includes all the z-normalized step rates within it, which serve as the input and output variables for chained equations. Additionally, we incorporate one-hot vectors representing day of the week and hour of the day for the center imputation instance as observed variables, which can only be conditioned on during training. Mathematically, we denote $x_i$ as the normalized step rate of some position $i$ in the context window, and let $x_{-i}$ be normalized step rates from all the other positions in the same context window. Also, $\mathbf{\theta}$ is the concatenation of two one-hot vectors for day of the week and hour of the day. Therefore, the prediction for $x_i$ is defined as: $\hat{x}_i = \mathtt{g}(x_{-i}, \mathbf{\theta}), i \in \{1,\ldots, I\}$, where $I$ is the number of positions in the context window and $\mathtt{g}$ is the linear regression in our case: $\mathtt{g}^{i}(x_i) = w^{i}x_{-i} + b^i$, where $\mathbf{\theta}$ is ignored for simplicity. 

To train our iterative imputation model, we set the initial normalized step rate value belonging to originally missing hourly blocks and test hourly blocks as zeros. We use 
\emph{sklean.linear\_model.SGDRegressor} with \emph{partial\_fit} method to train each linear regression model in the chained equation using mini-batch SGD with the batch size of 10,000 for 2 epochs. We initialize the learning rate as 0.001 and use the \emph{invscaling} scheduler implemented by sklean to conduct the learning rate decay. The loss function is epsilon insensitive loss with $\epsilon=0.01$. The number of imputation iterations is set as 2, so that before the second iteration, the missing values have already been filled by the first iteration. Also, weight decay with the coefficient 0.0001 is leveraged to regularize each linear regression model. We specify the imputation order of context window positions as alternating between the positions from the start and from the end, so that before filling the center hourly block, missing values of all the other positions in the context window have already been imputed. Figure \ref{fig:mice_order} provides an example. 

\begin{figure}[ht]
\centering
\includegraphics[width=0.8\columnwidth]{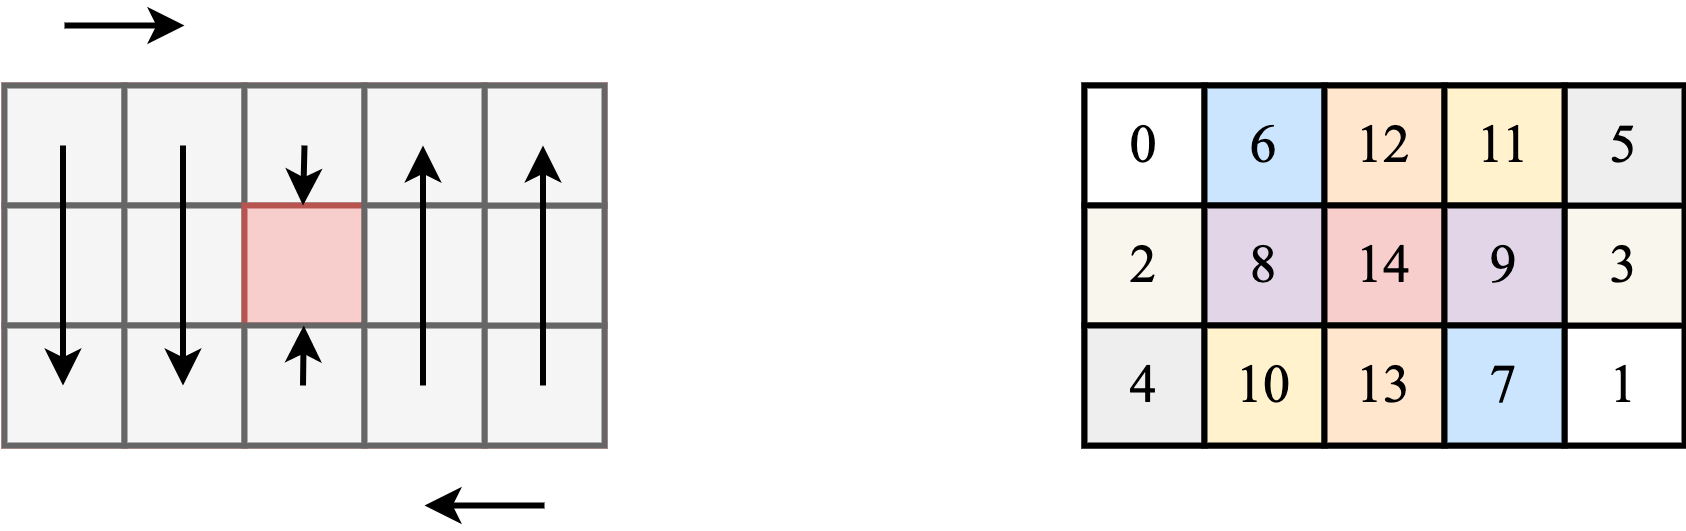}
\caption{The order of prediction positions within the local context window using iterative imputations. The order is alternating between the start (i.e. upper left) and the end (i.e. lower right). The direction from the start is from top to bottom from left to right, while the direction from the end is from bottom to top, from right to left. The plot on the right gives an example. The number means the order of computation and the same color means the same relative position from the start and from the end.} 
\label{fig:mice_order}
\end{figure}

During inference, we perform multiple imputations for each position by sampling from a Gaussian distribution. The mean for the distribution is derived from a trained linear regression, and the variance is estimated from the average squared error between the predictions and the ground-truth values. Also, the sampled step rate will go through the same non-linearity used in other methods to limit its range within zero and 1.5 times maximum step rate from the same participant. In our experiment, we configure the number of samples as 5, and the final prediction for each position is based on the average of them. Algorithm \ref{alg:mi} illustrates the inference procedure with multiple imputation. 

\textbf{Step-by-step explanation of Algorithm \ref{alg:mi}:}

Line 0: before illustration, we need to reiterate: direct outputs from the model are \emph{z-normalized step rates} and we evaluate the model on \emph{step counts}. In the following, $SC$ means step counts, $sr$ or $SR$ means \emph{unnormalized} step rates, and $x$ is \emph{normalized} step rate.

Line 1: initialize a variable to record average \emph{step counts} sampled by the algorithm for the center position $I$ in a context window from participant $n$.

Line 2 and 3: the outer for-loop is for sampling, the inner for-loop is to iterate every position in the context window with the order in Figure \ref{fig:mice_order}. $I$ is the last position, which is the center of the local window. 

Line 4: draw a sample for position $i$ from Gaussian distribution with zero mean. The variance is estimated by the mean square error between predicted values from the linear regression $\mathtt{g}$ and true z-normalized step rate values at position $i$ over the entire validation or test set. The variance is shared across position $i$ in local context windows from all the participants.

Line 5: use the linear regression and the sampled noise to get the normalized step rate at position $i$ in a context window from participant $n$. We limit the range of predicted \emph{unnormalized} step rates between zero and 1.5 fold maximum step rate in the training dataset of participant $n$. Here, we convert this range into the \emph{normalized} step rate level using personalized mean $\mu_{SR}^{(n)}$ and standard deviation $\sigma_{SR}^{(n)}$ derived from all the \emph{unnormalized} step rates from participant $n$.

Line 7: after predicting the normalized step rate for poisition $I$, we convert it back to the unnormalized step rate using the same personalized mean and standard deviation as above.

Line 8: Convert the normalized step rate into the step count within the same hourly block using wearing minutes $VM$. Record this sampled step count in the current iteration for later averaging.

%\textcolor{red}{TODO: add a figure to show the imputation order and add a paragraph to explain the algorithm}

%% This declares a command \Comment
%% The argument will be surrounded by /* ... */
\SetKwComment{Comment}{/* }{ */}

\begin{algorithm2e}
\caption{Inference with Multiple Imputations}\label{alg:mi}
%\KwData{$n \geq 0$}
%\KwResult{$y = x^n$}
%$y \gets 1$\;
%$X \gets x$\;
%$N \gets n$\;
% \While{$N \neq 0$}{
%   \eIf{$N$ is even}{
%     $X \gets X \times X$\;
%     $N \gets \frac{N}{2}$ \Comment*[r]{This is a comment}
%   }{\If{$N$ is odd}{
%       $y \gets y \times X$\;
%       $N \gets N - 1$\;
%     }
%   }
% }
$SC^{(n)}_{I} \gets 0$ \;
  \For{$s\gets1$ \KwTo $S$}{
    \For{$i\gets1$ \KwTo $I$}{
    $\epsilon_{i,s} \sim \mathcal{N}(0,\sigma_{i}^{2})$ \Comment*[r]{$\sigma^{2}_{i}\approx \frac{1}{m_{i}}\sum_{m=1}^{M_{i}}\|\hat{x}_{i,m}- x_{i,m}^{true}\|^{2}$}\
    $\hat{x}^{(n)}_{i,s} \gets \mathtt{P}(w^ix^{(n)}_{-i} + b^i + \epsilon_{i,s})$ \Comment*[r]{ $\mathtt{P}(x^{(n)}) = \max(-\frac{\mu^{(n)}_{SR}}{\sigma^{(n)}_{SR}}, \min(x, \frac{1.5 \max {sr}^{(n), train}-\mu^{(n)}_{SR}}{\sigma^{(n)}_{SR}}))$}
    
    }
$\hat{sr}^{(n)}_{I} = \hat{x}^{(n)}_{I} \times \sigma^{(n)}_{SR} + \mu^{(n)}_{SR}$ \;
$SC_{I} \gets SC_{I} + \frac{1}{S}\hat{sr}_{I} \times VM_{I}$
}

\end{algorithm2e}

\subsection{Convolutional Denoise Autoencoder (CNN-DAE)}
We use the symmetric encoder-decoder architecture to implement CNN-DAE. The encoder consists of three 1D convolutional layers, each followed by BatchNorm and ReLU activation. Similarly, the decoder includes three 1D transposed convolutional layers, with the first two layers being followed by Batch Normalization and ReLU activation. The configurations of convolutional and transposed convolutional layers are in Table \ref{tab:conv_config}.

\begin{table}[h!]
\caption{Configurations for Convolutional and Transpose Convolutional Layers in CNN-DAE}
\small
\centering
\resizebox{\columnwidth}{!}{%
\begin{tabular}{@{}llllll@{}}
\toprule
\textbf{Layer} & \textbf{Input Channels} & \textbf{Output Channels} & \textbf{Kernel Size} & \textbf{Stride} & \textbf{Padding} \\ \midrule
Conv1      & 2  & 4  & 31 & 2 & 11 \\
Conv2      & 4  & 8  & 20 & 2 & 9  \\
Conv3      & 8  & 16 & 10 & 2 & 4  \\ \midrule
TransConv1 & 16 & 8  & 10 & 2 & 4  \\
TransConv2 & 8  & 4  & 20 & 2 & 9  \\
TransConv3 & 4  & 2  & 31 & 2 & 11 \\ \bottomrule
\end{tabular}%
}
\label{tab:conv_config}
\end{table}

For the input, we include both z-normalized step rates and heart rates within the same local context window used in other model-based methods. \textcolor{red}{Since the CNN model structure is not suitable for use with the multi-scale context window, we apply it at the hourly level to the contiguous time span from the first to last hourly block in the context window used by the proposed model. Furthermore, LAPR is not employed in CNN-DAE due to its inability to yield better performance.}

During training, we set as zeros all the hourly blocks belonging to (1) the center of each context window (i.e. what we are actually imputing for) (2) the test set (3) positions which are originally missing in the participant data. We calculate the MAE loss between reconstructed and ground-truth z-normalized step rates of all the hourly blocks belonging to the training set. 

Also, we consider the heart rate reconstruction as the auxiliary task and minimize the combined reconstruction MAE loss on step rates and heart rates as $\text{total loss}= \text{MAE(step rates)} + \lambda \text{MAE(heart rates)}$. We search for $\lambda$ within \{0.0, 0.5, 1.0\}. However, since our final goal is to reconstruct the step count of the center hourly block of each local context window, we compute the MAE on step counts over all the center hourly blocks belonging to the validation set to select the best hyperparameters and conduct the early stopping. 

We use Adam optimizer and set the batch size as 50,000 to train the model of each split for 20 epochs. The learning rate is searched within \{0.1, 0.01, 0.001\}.  

\subsection{BRITS} \label{sec:brits}
% We follow the same setting of the original paper, which leverages LSTM as the RNN architecture. The input features are from hourly blocks within the same multi-timescale context window used for other models as a fair comparison. The context window is flattened in the chronological order so that RNN model can process them step-by-step.  We impute both heart rates and step rates at each time step and use BRITS loss, which is the summation of the reconstruction loss (i.e. MAE) and the consistency loss (i.e. makes forward and backward LSTM have the consistent prediction at each step), to train the model. We note BRITS loss in our case is at the normalized step rate and normalized heart rate level. During validation, we monitor the validation loss, which is the Micro MAE computed on the \emph{step count} level over all the testing hourly blocks. This is because our final task is to impute the step counts rather than the step rates or normalized step rates. We conduct the early stopping and select the best hyperparameters based on the best validation loss. We train the BRITS model for 30 epochs with the batch size of 10,000 and the learning rate of 0.01. The LSTM hidden state dimension is searched within \{4, 8, 16, 32\}.

We adhere to the settings outlined in the original paper, utilizing LSTM as the RNN architecture. Input features are derived from hourly blocks within the same multi-timescale context window, ensuring a fair comparison with other models. \textcolor{red}{Moreover, we found LAPR cannot help to improve performance, thus we did not use it here.} The context window is chronologically flattened, enabling the RNN model to process information sequentially.

We impute both heart rates and step rates at each time step, utilizing the BRITS loss, which is a combination of the reconstruction loss (i.e., MAE) and the consistency loss (i.e., ensuring forward and backward LSTM predictions consistent at each step). Notably, our BRITS loss is at the \emph{normalized step rate} and \emph{normalized heart rate} level. \textcolor{red}{Notebly, we found that the auxiliary heart rate imputation task indeed helps the step rate imputation task for BRITS, so we keep both of them during training.}
Validation involves monitoring the Micro MAE, computed on the \emph{step count} level across all the validation hourly blocks. This choice is reflective of our ultimate task, which centers on imputing step counts rather than step rates or normalized step rates. Early stopping is implemented, and the best hyperparameters are selected based on the optimal validation loss.

Training the BRITS model spans 30 epochs with a batch size of 10,000 and a learning rate of 0.01. The LSTM hidden state dimension is searched within \{4, 8, 16, 32\}.

\subsection{MRNN}
% MRNN consists of an interpolation block and an imputation block. In the interpolation block, we apply two bidirectional-GRU models to interpolate the missing values in step rates and heart rates. Since the interpolation block computes the missing values within each data stream, the day of the week and hour of the day one-hot vectors, which are always observed, are not input into the model. In the imputation block, since MRNN impute the missing values across different variables, we input day of the week and hour of the day features here. During training, train/valid and test visibility and the context window is the same as these in the self-attention model, but same as BRITS, the context window is flattened in the chronological order for the RNN to process. To keep consistent with other models, we use MAE instead of MSE to train the model, which is different from the original paper. We train MRNN for 40 epochs, with the batch size of 20,000 and the learning rate of 0.01. GRU hidden state dimension is searched within \{4, 8, 16, 32\}. 

MRNN comprises an interpolation block and an imputation block. In the interpolation block, we employ two bidirectional-GRU models to fill in missing values in step rates and heart rates. Given that the interpolation block calculates missing values within each data stream, day of the week and hour of the day one-hot vectors, which are always observed, are excluded from the model input. In the imputation block, as MRNN handles missing values based on information across different variables, we include day of the week and hour of the day features in the input features. 

During training, the visibility of train/valid and test sets, along with the context window, aligns with that in the self-attention model. \textcolor{red}{As suggested by the original paper, we fill the missing values outside of the center hourly block with zeros. Moreover, we found that DW+HD median filling does not demonstrate the performance as good as zero-filling.} Like BRITS, the context window is flattened in chronological order for RNN processing. \textcolor{red}{We also found LAPR can improve the MRNN performance as with our proposed model, thus these features are used when reporting the results.}

To keep consistent with other models, we employ Mean Absolute Error (MAE) instead of Mean Squared Error (MSE) for model training, different from the original paper. We train MRNN for 40 epochs, utilizing a batch size of 20,000 and a learning rate of 0.01. The GRU hidden state dimension is searched within \{4, 8, 16, 32\}.

\subsection{USGAN}
% We use the BRITS model as the generator and a bidirection-GRU model as the discriminator. The generator configurations are the same as stated in \sectionref{sec:brits}. Since our data has no label associated with each time series, we ignore the classifier in the original paper. Unlike the original implementation which updates the discriminator five times after the generator is updated, we found updating the discriminator once can generate more stable training and a better performance in our case. 

% We train the USGAN for 30 epochs with the batch size of 10,000 and the learning rate of 0.01. The RNN hidden state dimension for generator and discriminator are searched within \{4, 8, 16, 32, 64\}. The weight of the discriminator loss during training, which balances the discriminator loss and BRITS loss, is searched within{\0.1, 0.3, 0.5, 0.7, 0.9, 1.0\}.

We employ the BRITS model as the generator and a bidirectional GRU model as the discriminator. The generator configurations align with those outlined in \sectionref{sec:brits}. As our data does not have labels for each time series, we omit the classifier mentioned in the original paper. In contrast to the original implementation, which updates the discriminator five times after each generator update, we observe that updating the discriminator only once results in more stable training and improved performance in our case.

We train the USGAN model for 30 epochs with a batch size of 10,000 and a learning rate of 0.01. The RNN hidden state dimensions for both the generator and discriminator are explored within \{4, 8, 16, 32, 64\}. Additionally, we search for the weight of the discriminator loss during training, which balances it and BRITS loss, within \{0.1, 0.3, 0.5, 0.7, 0.9, 1.0\}.

\subsection{\textcolor{red}{SAITS}}
\textcolor{red}{We use a learning rate of 0.01 and batch size of 10,000 when training the model. We fix the number of transformer layers at 2 and search for the hidden representation dimension $d_{model}$ and the output dimension from each layer $d_v$ within \{4, 8, 16, 32\} using our validation set. We applied SAITS with the same multi-scale context window used by our approach as well as the same features (note that SAITS uses dense self-attention, which is not feasible for our data due to the average time series length).}

\subsection{Computing Infrastructure} \label{sec:comp_infra}
We use Faiss-cpu \footnote{https://github.com/facebookresearch/faiss} to search for $k$-nearest neighbors. Iterative imputation method is implemented using scikit-learn v1.0.2. Regression Imputation, CNN-DAE, Self-Attention, BRITS, MRNN and USGAN are implemented using PyTorch v1.13.1 and trained with NVIDIA Tesla T4 GPUs provided in the  \textit{All of Us} workspace. 

%\clearpage

\section{Formal Definitions of Evaluation Metrics} \label{sec:eval_metrics}
Let $m_n \in \mathcal{M}^{(n)}$ indicates the index of a single hourly block to be imputed from participant $n$ in either train, valid or test set. Then, Micro and Macro MAE and RMSE are defined as below: 

\begin{align*}
&\textit{Micro MAE} = \frac{1}{\sum_{n} \sum_{m_{n}} 1} \sum_{n=1}^{N} \sum_{m_n=1}^{|\mathcal{M}^{(n)}|} AE_{n,m_n}\\
&\textit{Macro MAE} = \frac{1}{N} \sum_{n=1}^{N} \frac{1}{|\mathcal{M}^{(n)}|} \sum_{m_n=1}^{|\mathcal{M}^{(n)}|} AE_{n,m_n} \\
&\textit{Micro RMSE} = \sqrt{\frac{1}{\sum_{n} \sum_{m_n} 1} \sum_{n=1}^{N} \sum_{m_n=1}^{|\mathcal{M}^{(n)}|} SE_{n,m_n}} \\
&\textit{Macro RMSE} = \frac{1}{N} \sum_{n=1}^{N} \sqrt{\frac{1}{|\mathcal{M}^{(n)}|} \sum_{m_n=1}^{|\mathcal{M}^{(n)}|} SE_{n,m_n}}
\end{align*}

where $N$ is the number of participants in the dataset and $|\mathcal{M}^{(n)}|$ is the number of imputed hourly blocks from participant $n$. 

%\clearpage

\section{Imputation Results on Test sets from Stratified Sampling Splits}
\tableref{tab:results} shows the imputation results of four evaluation metrics on the test sets from 10 stratified sampling splits. Each result shows the mean and standard deviation over 10 splits. For each model category, we run two-sided student t-test and emphasize results which are better than others with statistical significance ($p<0.05$) on each evaluation metric. The red color indicates the model with the overall best performance (i.e. sparse self-attention model), which is better than the second best model (i.e. regression imputation) with statistical significance on all metrics ($p < 0.001$).

%\hwnote{we need to change trainable model --> model based methods}
%\hwnote{mulitple-imputation --> iterative imputation}

% Please add the following required packages to your document preamble:
% \usepackage{booktabs}
% \usepackage{multirow}
% \usepackage{graphicx}
\begin{table*}[]
\small
\caption{Imputation results of mean and standard deviation for each metric over 10 in-domain test splits}
\centering
\resizebox{0.9\textwidth}{!}{%
\begin{tabular}{@{}llcccc@{}}
\toprule
\textbf{Method Category} & \textbf{Method} &\textbf{Macro MAE} &  \textbf{Micro MAE} & \textbf{Macro RMSE} & \textbf{Micro RMSE} \\ \midrule
\multirow{4}{*}{Basic Fill}
 & Zero Fill & 602.40 ± 2.38 & 603.60 ± 2.41 & 1008.38 ± 4.17 & 1082.99 ± 4.55\\
 & Forward Fill & 542.50 ± 2.79 & 543.18 ± 2.85 & 939.49 ± 4.70 &  1011.39 ± 5.67\\
 & Backward Fill & 533.55 ± 1.50 & 534.27 ± 1.55 & 927.84 
± 4.15 & 997.77 ± 3.99\\
 & Avg. F+B Fill & \textbf{457.33 ± 1.89} & \textbf{457.91 ± 1.91} & \textbf{762.65 ± 2.82} & \textbf{818.33 ± 3.39}\\ \midrule
\multirow{4}{*}{Micro Mean Fill}
 & Participant & 526.57 ± 1.42 & 527.72 ± 1.43 & 803.63 ± 3.55 & 868.02 ± 3.94\\
 & Day of Week & 524.64 ± 1.43 & 525.78 ± 1.44 & 801.60 ± 3.54 & 865.81 ± 3.95\\
 & Hour of Day & 464.56 ± 1.69 & 465.32 ± 1.71 & 741.50 ± 3.28 & 796.71 ± 3.58\\
 & DW+HD & \textbf{449.06 ± 1.85} & \textbf{449.90 ± 1.88} & \textbf{725.04 ± 3.41} & \textbf{779.03 ± 3.79} \\ \midrule
\multirow{4}{*}{Mean Fill}
 & Participant & 528.74 ± 1.41 & 529.89 ± 1.41 & 803.75 ± 3.54 & 868.15 ± 3.92\\
 & Day of Week & 526.76 ± 1.41 & 527.91 ± 1.42 & 801.73 ± 3.52 & 865.94 ± 3.93\\
 & Hour of Day & 466.62 ± 1.68 & 467.37 ± 1.70 & 741.75 ± 3.25 & 796.93 ± 3.56\\
 & DW+HD & \textbf{450.94 ± 1.84} & \textbf{451.78 ± 1.87} & \textbf{725.35 ± 3.38} & \textbf{779.31 ± 3.75} \\ \midrule
\multirow{4}{*}{Median Fill}
 & Participant & 468.07 ± 1.86 & 469.15 ± 1.88 & 846.04 ± 4.03 & 917.75 ± 4.48 \\
 & Day of Week & 466.52 ± 1.85 & 467.59 ± 1.88 & 844.09 ± 4.02 & 915.65 ± 4.49 \\
 & Hour of Day & 418.84 ± 1.82 & 419.65 ± 1.86 & 782.77 ± 3.79 & 843.77 ± 4.15 \\
 & DW+HD & \textbf{407.13 ± 1.90} & \textbf{407.93 ± 1.94} & \textbf{764.14 ± 3.77} & \textbf{823.52 ± 4.15}\\ \midrule
\multirow{2}{*}{$k$NN}
 & Uniform & 403.53 ± 1.41 & 404.26 ± 1.44 & 683.09 ± 2.92 & 730.92 ± 3.23\\
 & Softmax & \textbf{401.83 ± 1.44} & \textbf{402.55 ± 1.48} & 680.16 ± 3.02 & \textbf{727.31 ± 3.37}\\ \midrule
\multirow{6}{*}{Model-based}
 & CNN-DAE \citep{jang2020deep} & 402.92 ± 1.89 & 403.60 ± 1.91 & 722.96 ± 6.17 & 776.95 ± 6.86\\
 & Iterative Imputation & 387.23 ± 1.50 & 387.92 ± 1.54 & 677.61 ± 3.08 & 726.23 ± 3.38 \\
 & Regression Imputation & 382.19 ± 1.60 & 382.85 ± 1.64 & 673.34 ± 3.04 & 721.01 ± 3.44\\
 & USGAN \citep{miao2021generative} \ & 376.13 ± 1.97 & 376.70 ± 2.01 & 693.73 ± 4.25 & 742.39 ± 5.03 \\
 & BRITS \citep{cao2018brits} & 375.63 ± 1.80 & 376.19 ± 1.85 & 692.67 ± 3.31 & 741.21 ± 3.83\\
 & MRNN \citep{yoon2018estimating} & 371.51 ± 1.90 & 372.08 ± 1.94 & 679.53 ± 4.17 & 725.85 ± 4.42 \\
 & Sparse Self-Attention (ours) & \textcolor{red}{\textbf{350.72 
± 1.40}} & \textcolor{red}{\textbf{351.32 ± 1.44}} & \textcolor{red}{\textbf{645.38 ± 3.90}} & \textcolor{red}{\textbf{689.09 ± 4.61}}\\ \bottomrule
 %& Self-Attention Model(d_k=4) & \textbf{352.58 (1.80)} & \textbf{353.21 (1.85)} & \textbf{646.45 (3.74)} & \textbf{689.82 (4.10)}\\ \bottomrule
\end{tabular}%
}
\label{tab:results}
\end{table*}

\section{Attention Mappings of Days of the Week} \label{sec:attn_alldayweeks}
\figureref{fig:attn_dayweek} shows the attention weights from our self-attention model when the predicted hourly block (i.e. center hourly block) belongs to each day of the week. For the comparison, we also attached the overall attention mapping at the end. 

\begin{figure*}[h!]
    \centering
    \includegraphics[width=1\linewidth]{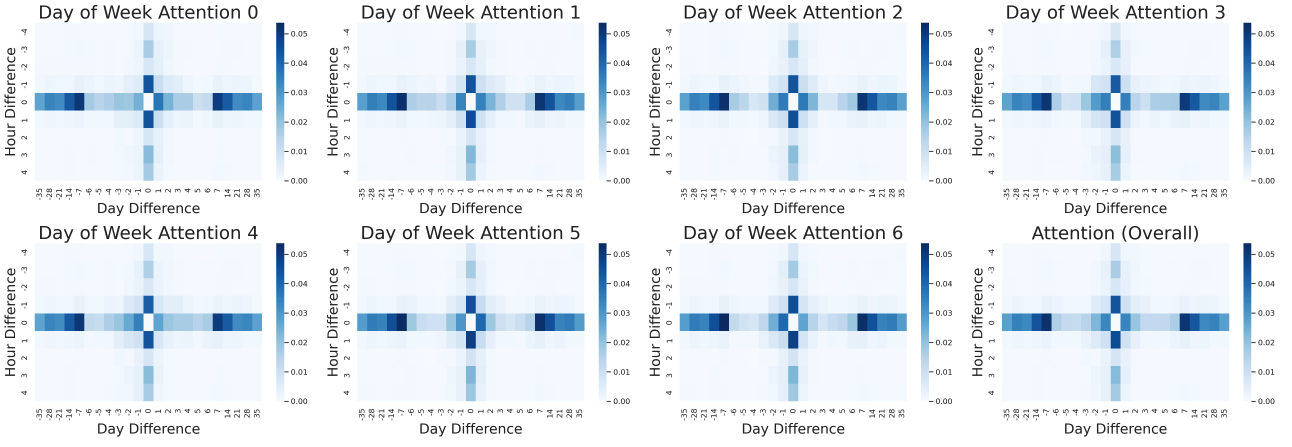}
    \caption{Visualization of attention weights of every day of the week. The overall attention weight is appended at the end for reference. All the attention weights are averaged over all completely held-out test samples.}
    \label{fig:attn_dayweek}
\end{figure*}

\section{\textcolor{red}{Autocorrelation Function of Heart Rate Data}}
\textcolor{red}{Figure \ref{fig:acf_hr} shows the autocorrelation function of heart rate data in \textit{All of Us} dataset. It demonstrates similar patterns as the step count data.}

\begin{figure}[t]
\includegraphics[width=\linewidth]{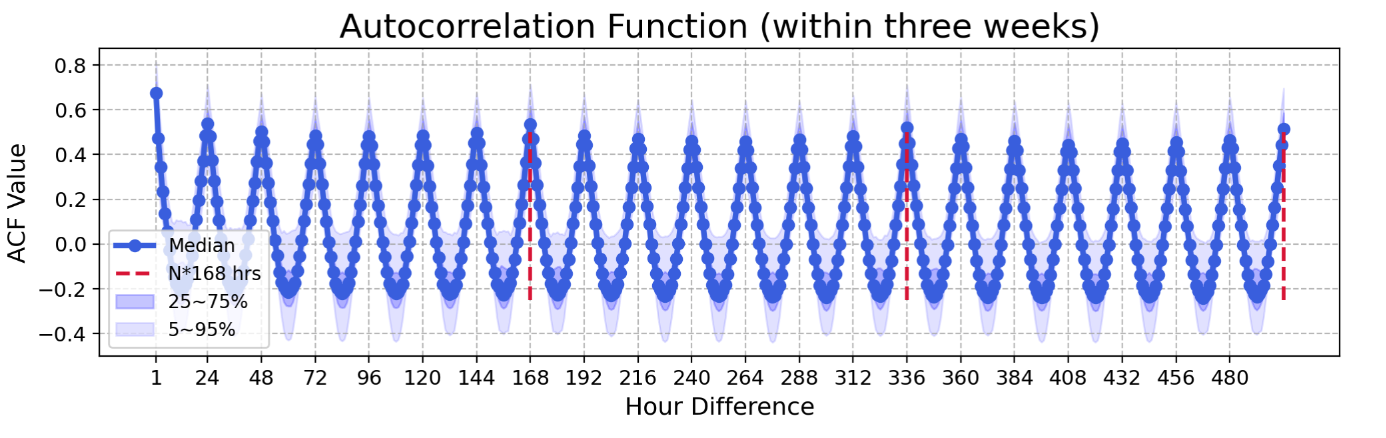}
\caption{Heart rate autocorrelation function (ACF) over all the participants within $\Delta t = 1, \ldots, 504$ hrs (within three weeks). \textbf{Blue line}: median ACF, \textbf{Red line}: $\Delta t=168 \times N$ hrs (i.e. $N$ weeks).}
\label{fig:acf_hr}
\end{figure}
